# Supplementary material for: Hardness of approximation for strip packing
Source: arXiv:1610.07766 source file (2016-10-25)
Supplement: Supplementary file 1 [file appendix.tex]

\appendix
\section{Appendix}

\subsection{Proof of Lemma \ref{lem:estimating-opt}}
TODO

\subsection{Proof of Lemma \ref{lem:rounding-verticals}}
TODO

\subsection{Proof of Lemma \ref{lem:delta-mu}}
TODO

\subsection{Proof of Lemma \ref{lem:moving-h-and-v}}
First, consider the horizontal items $H'$. As the number of boxes of the partition from Theorem \ref{thm:partition-1} is at most $K$, and each item is intersected along its longer edge, we get that $|H'| \le 2K / \delta$. Their total area is at most ...

TODO: finish (similar as in Lemma 3.3 on NW16)

Now, consider the vertical items $V'$. As previously, we get that $|V'| \le 2K / \delta$. The width of each of them is at most $\mu W$, so the total width is at most $\epsilon W$ if $\mu \le \frac{\epsilon \delta}{2 K}$. The number of different heights for all of them is at most $1/(\delta \epsilon)$, so we can group them into $1/(\delta \epsilon)$ boxes of equal-height items.
[similar as in Lemma 3.5 on NW16]
